# Supplementary material for: CoopReflect: Towards Natural Language Communication for Cooperative Autonomous Driving via Multi-Agent Learning
Source: arXiv:2505.18334 source file (2026-07-26)
Supplement: Supplementary file 1 [file appendix_qualitative_analysis.tex]

\section{Qualitative Analysis}
\label{sec:qualitative_analysis}
This section uses the \texttt{negotiation-highway-merge} scenario as an example scenario to analyze policy behaviors and qualitatively examines the learned knowledge and cooperation strategies. For detailed insights into the learned knowledge, please refer to \appref{appendix:qualitative-knowledge}, and refer to the supplementary videos for comprehensive demonstrations of policy behaviors.

% 1. message representation
First, we present a recorded communication exchange between agents in a demonstrative video:

\textcolor{mydarkblue}{\texttt{\textbf{Vehicle 121 (on the highway)}: Vehicle 120, I am slowing down to create a gap for your merge. Please proceed safely.}}

\textcolor{mydarkblue}{\texttt{\textbf{Vehicle 120 (merging) replied}: Thank you, Vehicle 121, I will speed up to merge into the gap you create. Please maintain your speed to facilitate my merge.}}

\textbf{This form of communication is human-interpretable}, paving the way for future human participation in multi-agent collaboration. In contrast, the $(x,y,z,feature)$ latent representation generated by Coopernaut lacks interpretability for humans and requires all vehicles in the collaboration system share the same encoder, limiting its flexibility in mixed-autonomy settings. While in this work we do not enforce that the communication be suitable for humans to participate in the collaboration directly, the results suggest that it may be possible to move in that direction in the future by enforcing short, real-time messages.

% 2. analyze learned knowledge
Second, the in-context knowledge developed through the debriefing process demonstrates a \textbf{clear and coherent cooperation strategy}, defining each agent's role and their coordination mechanisms (\appref{appendix:qualitative_highway_merge_negotiation}), in contrast to the purely reactive policies formed through self-reflection without explicit discussion of cooperation strategies (\appref{appendix:highway_merge_silent_tip_gpt}).

% 3. behavior analysis
Third, \textbf{agents behave according to their learned knowledge and cooperation strategy}.
In the \texttt{negotiation-highway-merge} scenario, the debriefing-based policy's behavior follows the developed structured cooperation strategy: when the merging vehicle requests to enter the highway, highway vehicles explicitly slow down to create a gap, enabling a smooth and coordinated merge. In contrast, under the \texttt{Correction+RAG (Silent)} mode, the lack in clear cooperation strategy leads to uncertainty. Both merging and highway vehicles struggle to determine the right of way, often resulting in either a collision or a prolonged indecisive interaction at the junction. We encourage readers to watch the supplementary videos accompanying this paper for a deeper understanding of the qualitative differences between policies.
