# Supplementary material for: CoopReflect: Towards Natural Language Communication for Cooperative Autonomous Driving via Multi-Agent Learning
Source: arXiv:2505.18334 source file (2026-07-26)
Supplement: Supplementary file 2 [file experiment_additional.tex]

\begin{table}[h!]
    \centering
    \caption{\small Experiment Results for Silent,  Zero-shot Comm and Debrief Comm Agents. We evaluate on adversarial cases where being aggressive or conservative will result in failure.}
    \resizebox{\textwidth}{!}{
    \begin{tabular}{lcc|ccc|ccc|ccc}
    \toprule
    \multicolumn{3}{c|}{\diagbox{Method}{Scenario}} & \multicolumn{3}{c|}{Overtake (Perception)} & \multicolumn{3}{c|}{Red Light} & \multicolumn{3}{c}{Left Turn} \\
    \midrule
    Name & LLM & Comm & 
    R $\uparrow$ & CR $\downarrow$ & SR $\uparrow$ & 
    R $\uparrow$ & CR $\downarrow$ & SR $\uparrow$ & 
    R $\uparrow$ & CR $\downarrow$ & SR $\uparrow$\\
    \midrule
     Zero-shot (Silent) & Yes & No & -1.00 & 1.00 & 0.0 & -0.40 & 0.70 & 30.0 & 0.06 & 0.43 & 53.3 \\
     Zero-shot (Comm) & Yes & Yes & -0.76 & 0.76 & 23.3 & 0.60 & 0.07 & 66.7 & 0.46 & 0.10 & 53.3 \\
    Debrief (Comm) & Yes & Yes & 0.43 & 0.26 & 70.0 & 0.76 & 0.00 & 76.7 & 0.86 & 0.03 & 90.0\\
    \midrule
    \multicolumn{3}{c|}{\diagbox{Method}{Scenario}} & \multicolumn{3}{c|}{Overtake (Negotiation)} & \multicolumn{3}{c|}{Highway Exit} & \multicolumn{3}{c}{Highway Merge} \\
    \midrule
     Zero-shot (Silent) & Yes & No & -1.86 & 1.93 & 3.3 & -1.73 & 1.86 & 6.7 & -2.00 & 2.00 & 0.0 \\
     Zero-shot (Comm) & Yes & Yes & 0.40 & 0.80 & 60.0 & -1.43 & 1.70 & 15.0 & -0.40 & 1.2 & 45.5 \\
    Debrief (Comm) & Yes & Yes & 0.73 & 0.50 & 51.6 & -0.16 & 0.93 & 38.3 & 0.96 & 0.50 & 73.3\\
    \bottomrule
    \end{tabular}
    }
    \label{tab:additional}
    \vspace{-6pt}
\end{table}
